# Supplementary material for: GRAM: Graph-based Attention Model for Healthcare Representation Learning
Source: arXiv:1611.07012 source file (2017-04-01)
Supplement: Supplementary file 1 [file appendix.tex]

\section{Generating GloVe Embeddings}
\label{appendix:glove}
\begin{figure}
%\floatbox[{\capbeside\thisfloatsetup{capbesideposition={left,center},capbesidewidth=7cm}}]{figure}[\FBwidth]	
{\caption{Creating the co-occurrence matrix together with the ancestors. Here we exclude the root node, which will be just a single row (column). We first create an augmented dataset by adding the ancestors of the code to the dataset. Then, we count the co-occurrence of the codes. Performing GloVe on this matrix produces the embedding vectors $\eb_i$.}
\label{fig:co-occur}}
{\quad\includegraphics[scale=0.28]{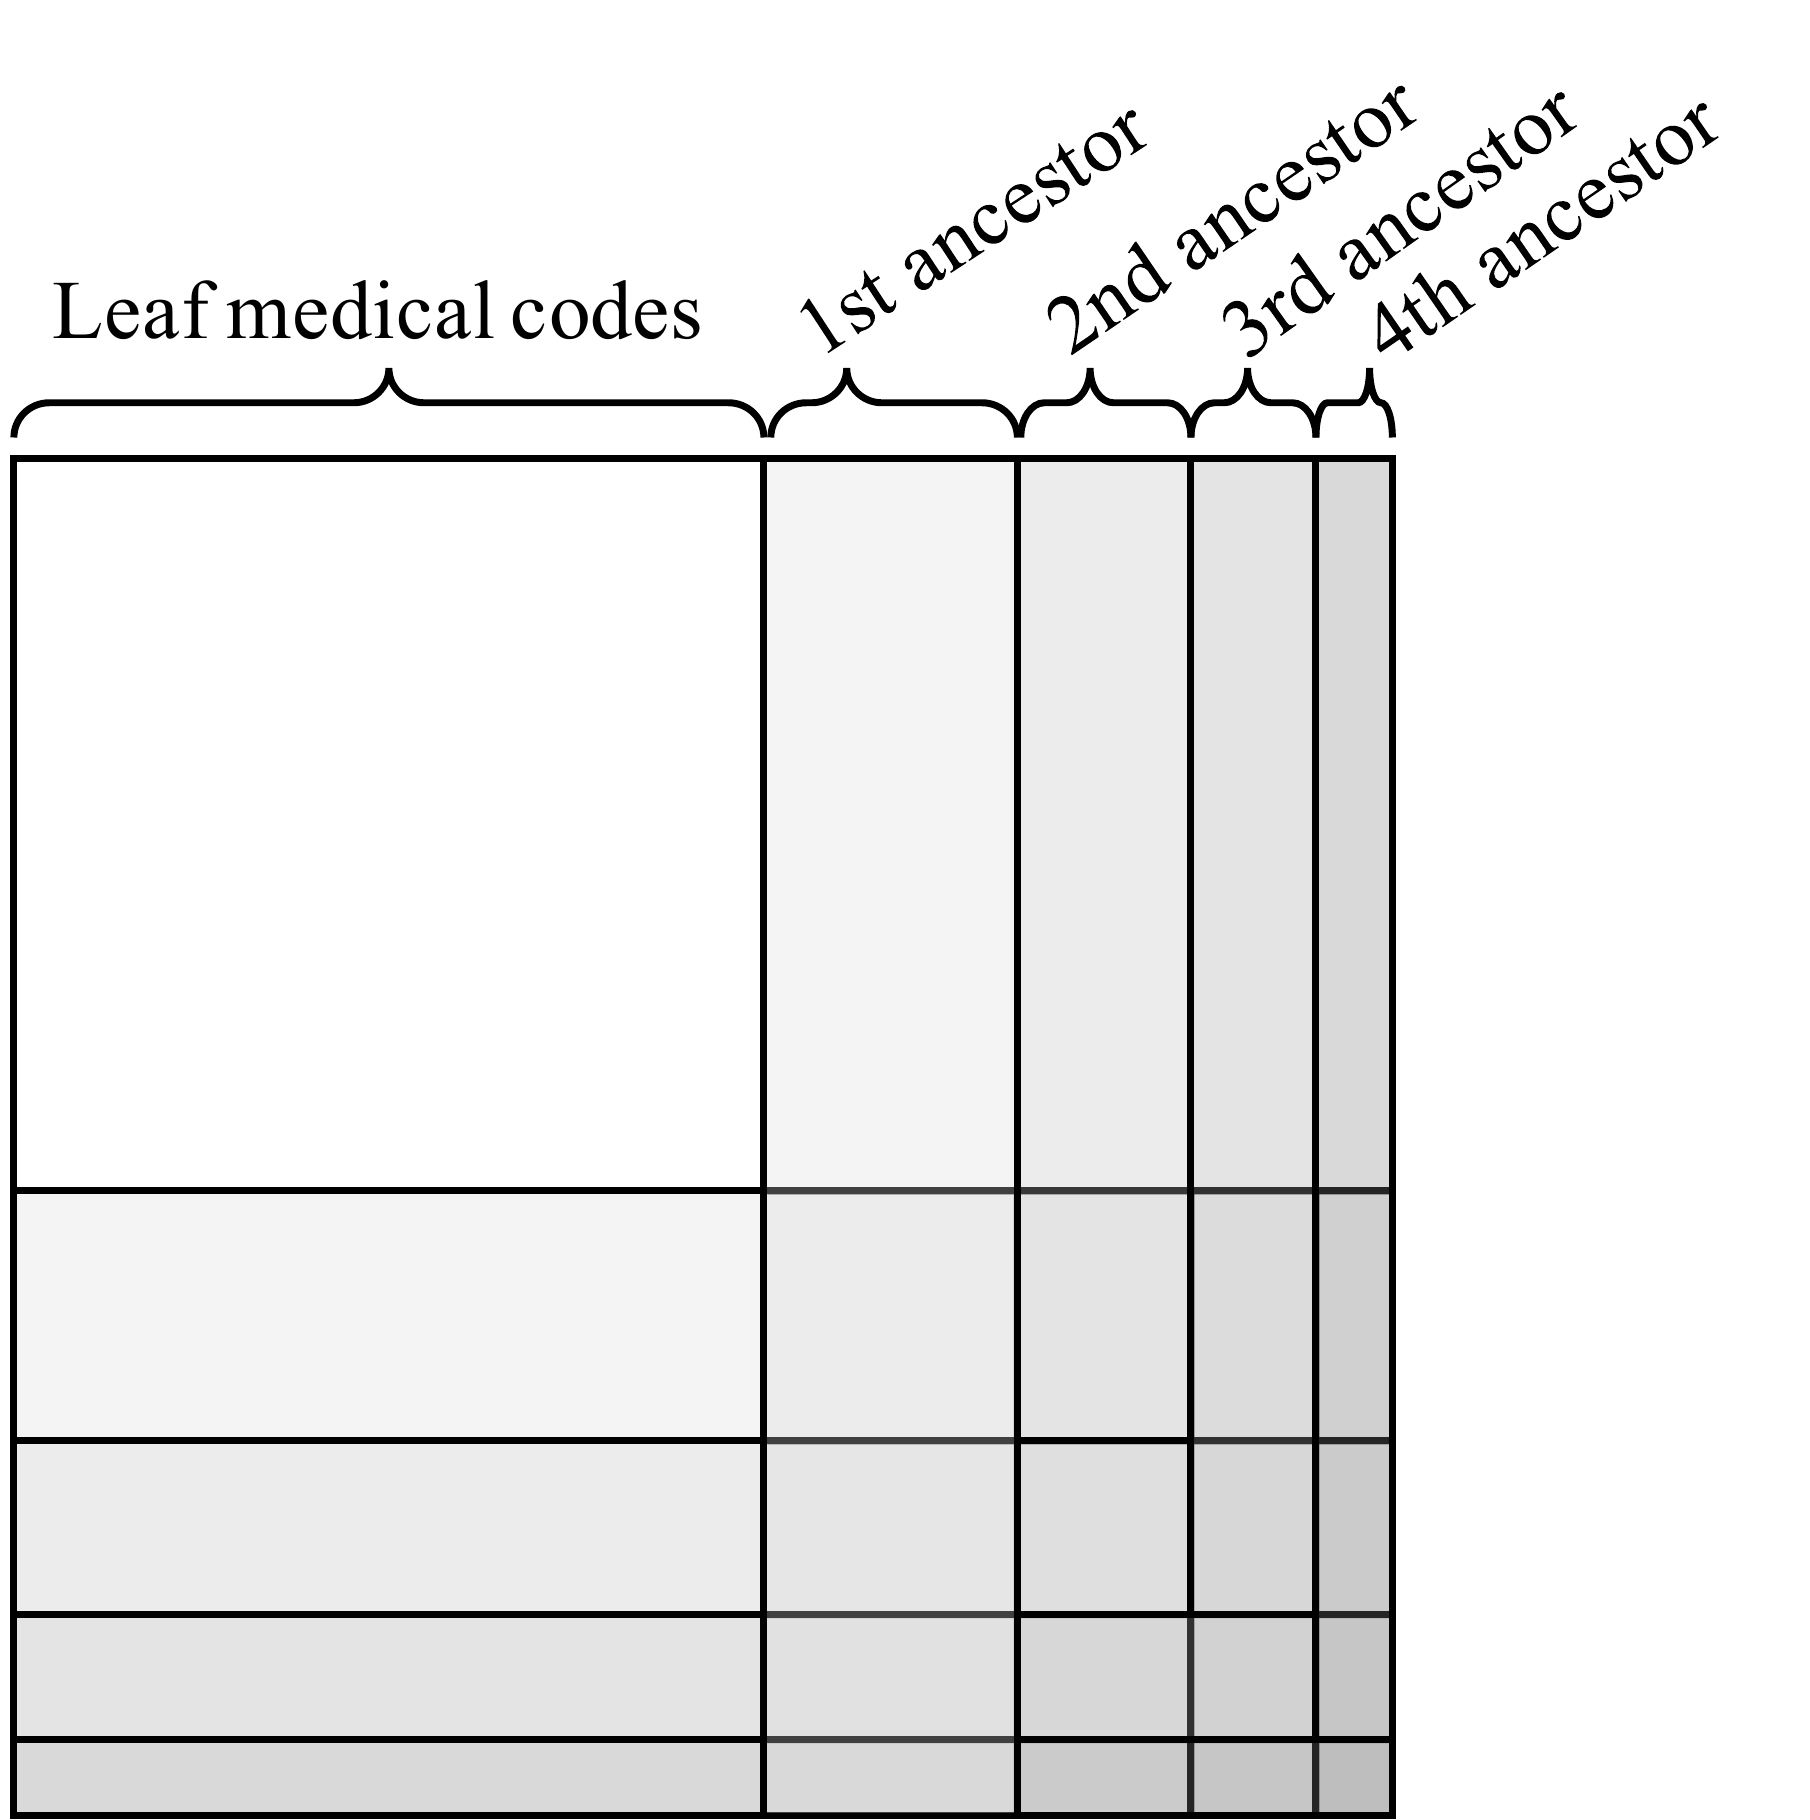}}  
\end{figure}
We learn the basic embeddings $\eb_i$'s of medical codes and their ancestors using GloVe \citep{pennington2014glove}, which uses global co-occurrence matrix of words to learn their representations. We generate the co-occurrence matrix of the codes and the ancestors by counting the co-occurrence within each visit $V_t$. However, since visits only contain the \textit{leaf} codes $c \in \mathcal{C}$, we augment each visit with the ancestors of the codes in each visit, then count the co-occurrence of codes and ancestors altogether.

We describe the details of the algorithm with an example. We borrow the parent-child relationships from the knowledge DAG of Figure \ref{fig:graph}. Given a visit $V_t$,
\begin{equation}
V_t = \{c_d, c_i, c_k\}
\end{equation}
we augment it with the ancestors of all the codes to obtain the augmented visit $V'_t$,
\begin{equation}
V'_t = \{c_d, \underline{c_b}, \underline{c_a}, c_i, \underline{c_g}, \underline{c_c}, \underline{c_a}, c_k, \underline{c_j}, \underline{c_f}, \underline{c_c}, \underline{c_b}, \underline{c_a}\}
\end{equation}
where the added ancestors are underlined. Note that a single ancestor can appear multiple times in $V'_t$. In fact, the higher the ancestor is in the knowledge DAG, the more times it is likely to appear in $V'_t$. We count the co-occurrence of two codes in $V'_t$ as follows,
\begin{equation}
co\mbox{-}occurrence(c_i, c_j, V'_t) = count(c_i, V'_t) \times count(c_j, V'_t)
\end{equation}
where $count(c_i, V'_t)$ is the number of times the code $c_i$ appears in the augmented visit $V'_t$. For example, the co-occurrence between the leaf code $c_i$ and the root $c_a$ is 3. However, the co-occurrence between the ancestor $c_c$ and the root $c_a$ is 6. Therefore our algorithm will naturally make the ancestor codes have higher co-occurrence with other codes compared to leaf medical codes. We repeat this calculation for all pairs of codes in all augmented visits of all patients to obtain the co-occurrence matrix depicted by Figure \ref{fig:co-occur}. For training the embedding vectors using the co-occurrence matrix, we use the same procedure and hyper-parameter as described in \citet{pennington2014glove}.

\section{Heart Failure Cohort Construction}
\label{appendix:cohort}
For the heart failure (HF) case patients, we select patients between 40 to 85 years of age at the time of HF diagnosis. HF diagnosis (HFDx) criteria are defined as: 1) Qualifying ICD-9 codes for HF appeared in the encounter records or medication orders. Qualifying ICD-9 codes are listed in Table \ref{table:hf_codes}. 2) at least three clinical encounters with qualifying ICD-9 codes had to occur within 12 months of each other, where the date of HFDx was assigned to the earliest of the three dates.  If the time span between the first and second appearances of the HF diagnosis code was greater than 12 months, the date of the second encounter was used as the first qualifying encounter.
Up to ten eligible controls (in terms of sex, age, location) were selected for each case, yielding average 9 controls per case. Each control was also assigned an index date, which is the HFDx date of the matched case. Controls are selected such that they did not meet the HF diagnosis criteria prior to the HFDx date plus 182 days of their corresponding case. Control subjects were required to have their first office encounter within one year of the matching HF case patient’s first office visit, and have at least one office encounter 30 days before or any time after the case’s HFDx date to ensure similar duration of observations among cases and controls. 

\begin{figure*}
\centering
\captionof{table}{Qualifying ICD-9 codes for heart failure}
\includegraphics[scale=0.6]{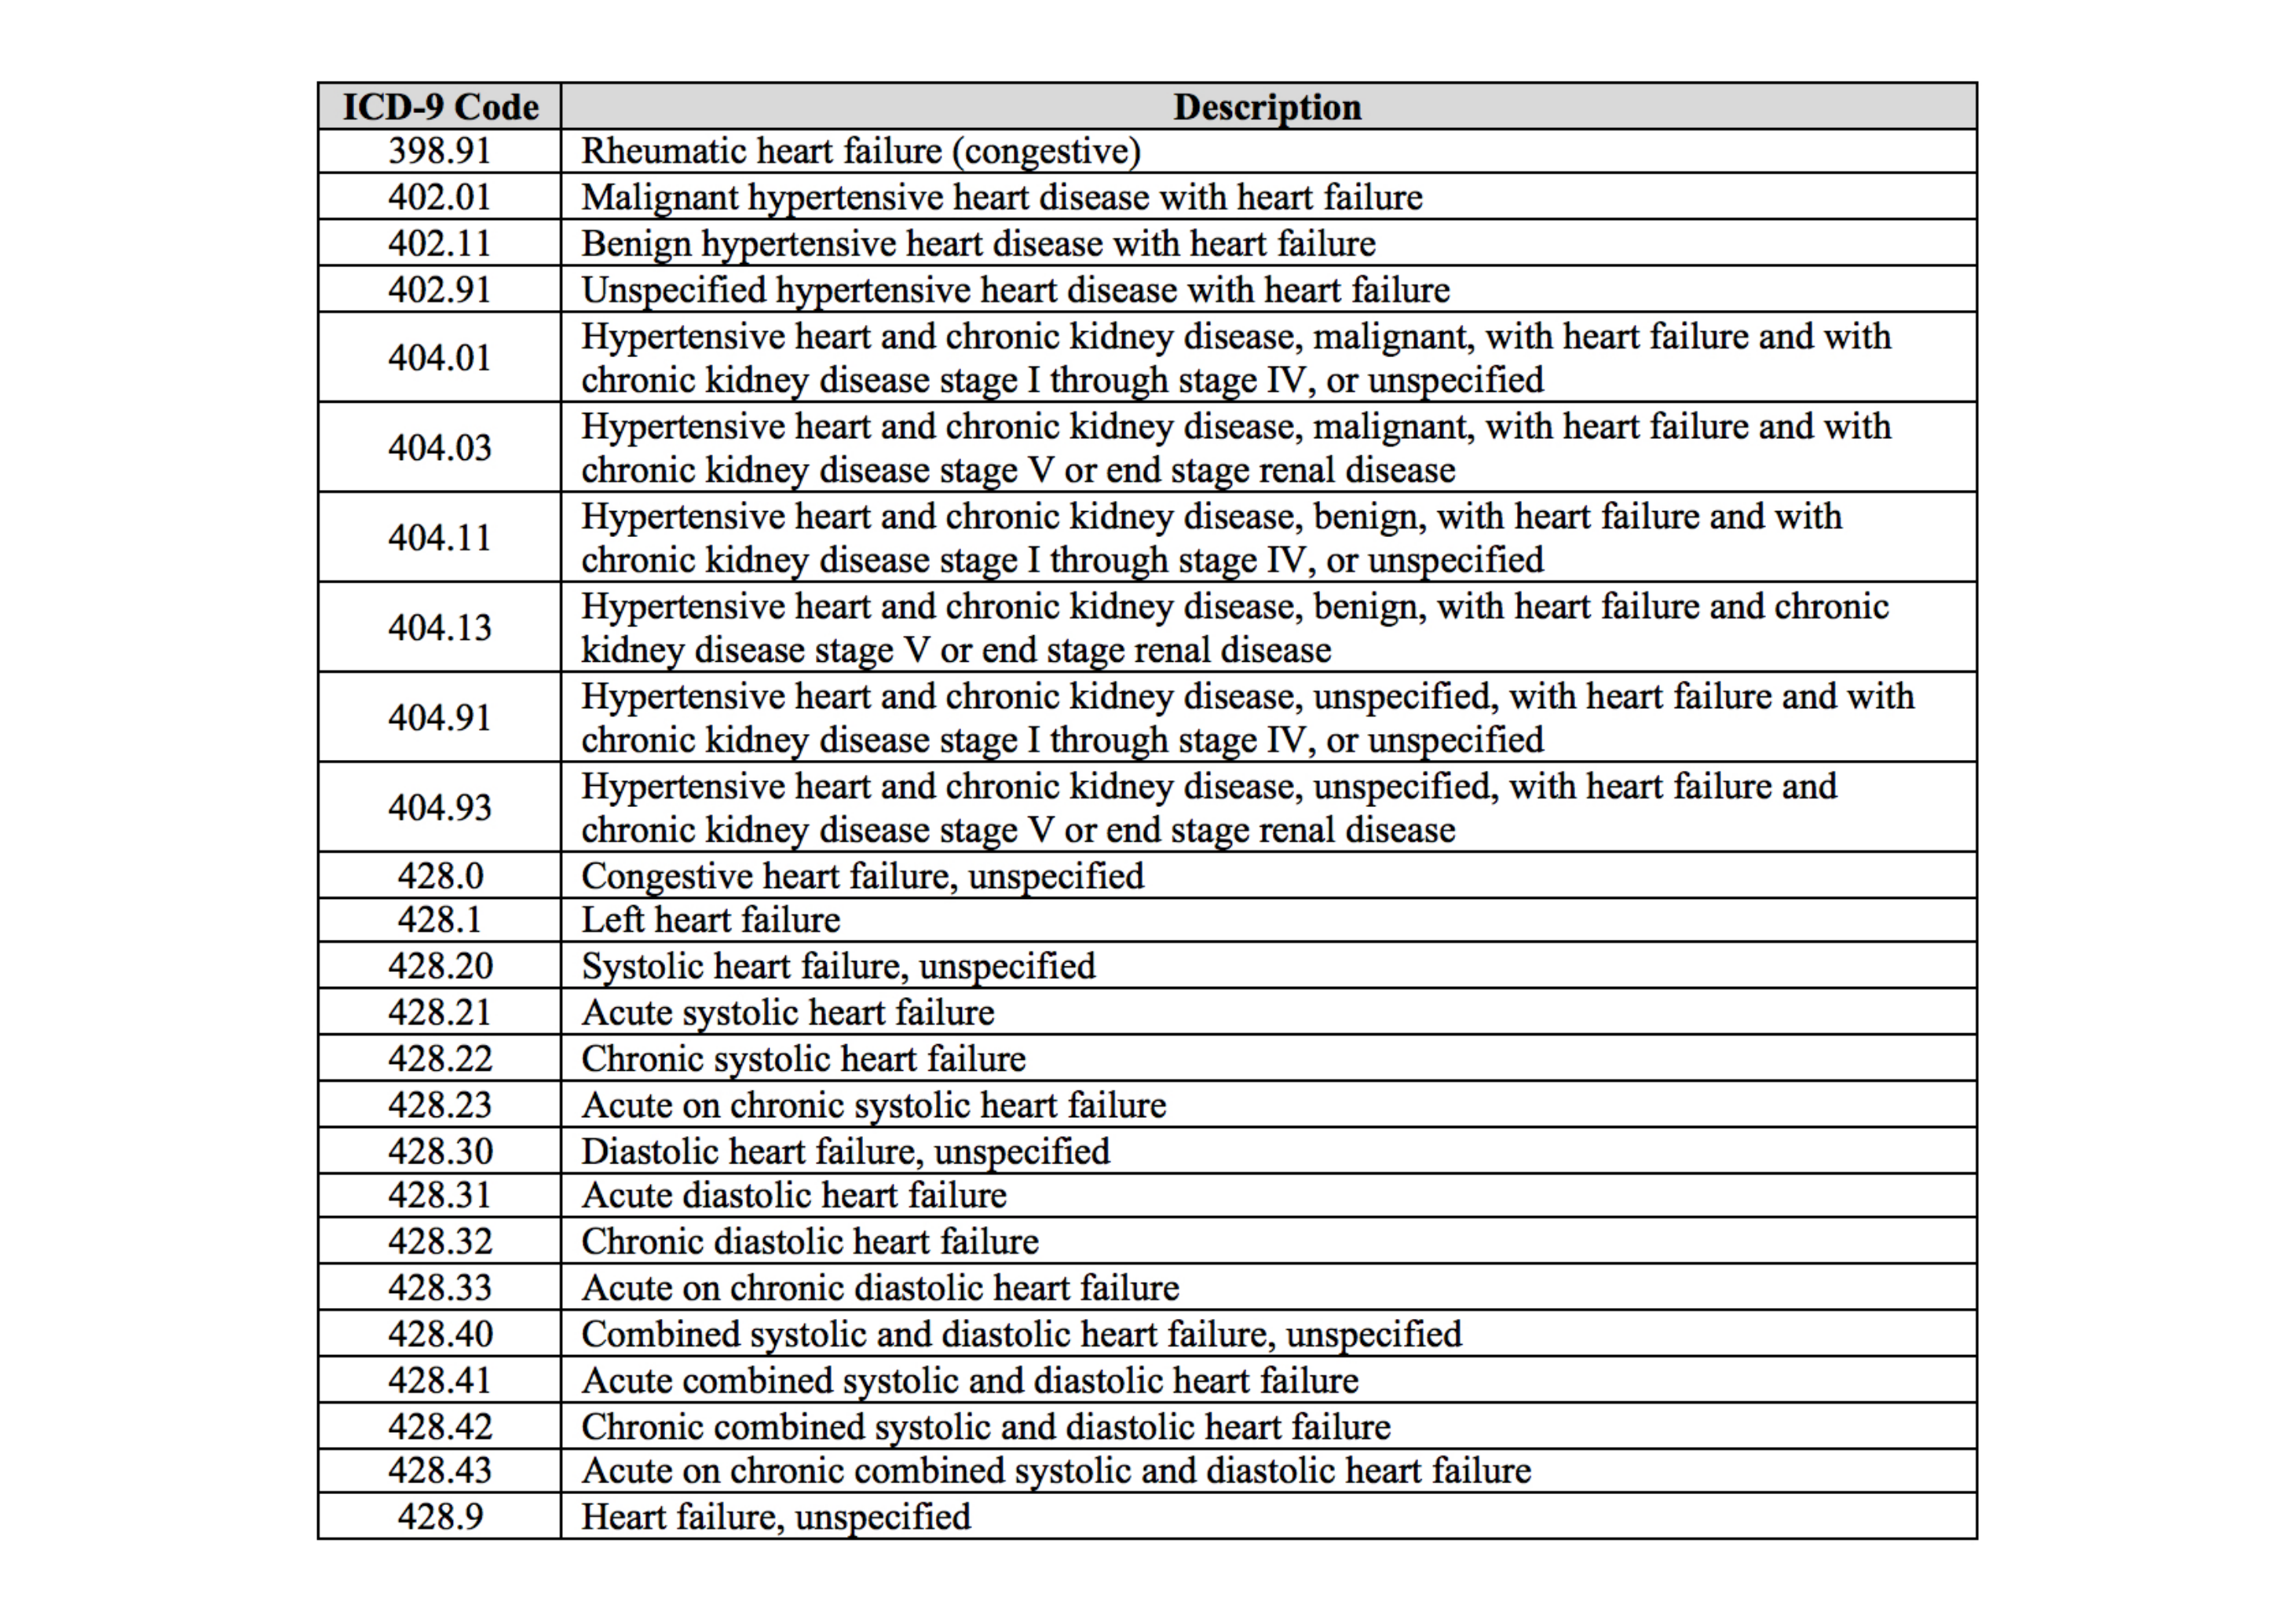}
\label{table:hf_codes}
\end{figure*}

\section{Hyper-parameter Tuning}
\label{appendix:hyperparameter}
\begin{table}[t]
\caption{Hyper-parameters used by the models in each predictive modeling experiments}
\label{tab:hyperparameter}
% \small
\vspace*{-2mm}
\centering
\begin{footnotesize}
\begin{tabular}{l|l|c|c|c|c|c}
\textbf{Experiment} & \textbf{Model} & $m$ & $r$ & $l$ & $L_2$ & Dropout rate \\ 
\toprule
\multirow{7}{*}{\begin{tabular}{l} Disease progression \\ modeling (Sutter data) \end{tabular}} & \texttt{GRAM}+ & 500 & 500 & 100 & 0.0001 & 0.6 \\ 
& \texttt{GRAM} & 500 & 500 & 100 & 0.0001 & 0.6 \\
& RandomDAG & 500 & 500 & 100 & 0.0001 & 0.6 \\
& RNN+ & 550 & 500 & & 0.0001 & 0.6 \\
& RNN & 550 & 500 & & 0.0001 & 0.6 \\
& SimpleRollUp & 500 & 500 & & 0.0001 & 0.4 \\
& RollUpRare & 500 & 500 & & 0.0001 & 0.2 \\
\midrule
\multirow{7}{*}{\begin{tabular}{l} Disease progression \\ modeling (MIMIC-III) \end{tabular}} & \texttt{GRAM}+ & 400 & 400 & 100 & 0.0001 & 0.6 \\ 
& \texttt{GRAM} & 400 & 400 & 100 & 0.001 & 0.6 \\
& RandomDAG & 400 & 400 & 100 & 0.001 & 0.6 \\
& RNN+ & 550 & 400 & & 0.001 & 0.8 \\
& RNN & 550 & 400 & & 0.001 & 0.8 \\
& SimpleRollUp & 400 & 400 & & 0.001 & 0.6 \\
& RollUpRare & 400 & 400 & & 0.0001 & 0.0 \\
\midrule
\multirow{7}{*}{\begin{tabular}{l} HF prediction \\ (Sutter HF cohort) \end{tabular}} & \texttt{GRAM}+ & 200 & 100 & 100 & 0.001 & 0.6 \\ 
& \texttt{GRAM} & 200 & 100 & 100 & 0.001 & 0.6 \\
& RandomDAG & 300 & 100 & 200 & 0.001 & 0.6 \\
& RNN+ & 200 & 100 & & 0.0001 & 0.6 \\
& RNN & 200 & 100 & & 0.001 & 0.6 \\
& SimpleRollUp & 300 & 200 & & 0.001 & 0.4 \\
& RollUpRare & 100 & 100 & & 0.001 & 0.6 \\
\bottomrule
\end{tabular}
\end{footnotesize}
\vspace{-4.3mm}
\end{table}
We define five hyper-parameters for \mname:
\begin{itemize}[leftmargin=5.5mm]
\item dimensionality $m$ of the basic embedding $\eb_i$: [100, 200, 300, 400, 500]
\item dimensionality $r$ of the RNN hidden layer $\hb_t$ from Eq. \eqref{eq:rnn_prediction}: [100, 200, 300, 400, 500]
\item dimensionality $l$ of $\Wb_a$ and $\bb_a$ from Eq. \eqref{eq:attention_function}: [100, 200, 300, 400, 500]
\item $L_2$ regularization coefficient for all weights except RNN weights: [0.1, 0.01, 0.001, 0.0001]
\item dropout rate for the dropout on the RNN hidden layer: [0.0, 0.2, 0.4, 0.6, 0.8]
\end{itemize}
We performed 100 iterations of the random search by using the above ranges for each of the three prediction experiments. For sequential diagnoses prediction on Sutter data, we used 10\% of the training data to tune the hyper-parameters to balance the time and search space.
To match the baselines' number of parameters to \mname's, we add 550 to the list of $m$'s possible values. This will make the baseline's largest possible number of parameters comparable to the \mname's largest possible number of parameters.

For SimpleRollUp and RollUpRare, the number of input codes is smaller than other models due to the grouping. Therefore, to match their largest possible number of parameters to \mname's, we need to add much larger values to $m$. However, after preliminary experiments, as expected, setting $m$ to too large a value degraded the performance due to overfitting. Since the number of input codes decreased due to the grouping, increasing the dimensionality of $\eb_i$ is not a logical thing to do. Therefore, for SimpleRollUp and RollUpRare, we use the same list of values for $m$ as other baselines.

Table \ref{tab:hyperparameter} describes the final hyper-parameter settings we used for all models for each prediction experiments.

\section{Prediction Results using Different $k$'s in Accuracy@k}
\label{appendix:prediction}
\begin{table*}
\centering
\small
%\vspace*{-2mm}
\begin{subtable}{1.\textwidth}
\centering
\begin{tabular}{l|c|c|c|c|c}
Model & 0-20 & 20-40 & 40-60 & 60-80 & 80-100\\ 
\toprule
GRAM+&\textbf{0.0150}&\textbf{0.3242}&0.4325&0.4238&0.4903\\
GRAM&0.0042&0.2987&0.4224&0.4193&0.4895\\
RandomDAG&0.0050&0.2700&0.4010&0.4059&0.4853\\
RNN+&0.0069&0.2742&0.4140&0.4212&\textbf{0.4959}\\
RNN&0.0080&0.2691&0.4134&0.4227&0.4951\\
SimpleRollUp&0.0085&0.3078&\textbf{0.4369}&\textbf{0.4330}&0.4924\\
RollUpRare&0.0062&0.2768&0.4176&0.4226&0.4956\\
\bottomrule
\end{tabular}
\caption{\textit{Accuracy@5} of sequential diagnoses prediction on Sutter data}
\label{tab:sdp_sutter_5}
\end{subtable}

\begin{subtable}{1.\textwidth}
\centering
\begin{tabular}{l|c|c|c|c|c}
Model & 0-20 & 20-40 & 40-60 & 60-80 & 80-100\\ 
\toprule
GRAM+&\textbf{0.0319}&\textbf{0.3882}&0.5054&0.5215&0.6459\\
GRAM&0.0163&0.3645&0.4944&0.5173&0.6445\\
RandomDAG&0.0142&0.3285&0.4691&0.5025&0.6401\\
RNN+&0.0183&0.3412&0.4884&0.5233&\textbf{0.6538}\\
RNN&0.0196&0.3290&0.4871&0.5230&0.6531\\
SimpleRollUp&0.0164&0.3768&\textbf{0.5132}&\textbf{0.5326}&0.6521\\
RollUpRare&0.0204&0.3450&0.4917&0.5228&0.6535\\
\bottomrule
\end{tabular}
\caption{\textit{Accuracy@10} of sequential diagnoses prediction on Sutter data}
\label{tab:sdp_sutter_10}
\end{subtable}

\begin{subtable}{1.\textwidth}
\centering
\begin{tabular}{l|c|c|c|c|c}
Model & 0-20 & 20-40 & 40-60 & 60-80 & 80-100\\ 
\toprule
GRAM+&\textbf{0.0630}&0.4486&0.5764&0.6153&0.7973\\
GRAM&0.0442&0.4276&0.5669&0.6125&0.7963\\
RandomDAG&0.0397&0.3933&0.5389&0.5997&0.7919\\
RNN+&0.0483&0.4132&0.5654&0.6235&0.8003\\
RNN&0.0481&0.4025&0.5630&0.6232&0.7995\\
SimpleRollUp&0.0418&\textbf{0.4496}&\textbf{0.5877}&\textbf{0.6262}&\textbf{0.8013}\\
RollUpRare&0.0517&0.4170&0.5672&0.6214&0.8002\\
\bottomrule
\end{tabular}
\caption{\textit{Accuracy@20} of sequential diagnoses prediction on Sutter data}
\label{tab:sdp_sutter_20}
\end{subtable}

\begin{subtable}{1.\textwidth}
\centering
\begin{tabular}{l|c|c|c|c|c}
Model & 0-20 & 20-40 & 40-60 & 60-80 & 80-100\\ 
\toprule
GRAM+&\textbf{0.0946}&0.4879&0.6186&0.6792&\textbf{0.8800}\\
GRAM&0.0662&0.4693&0.6107&0.6766&0.8798\\
RandomDAG&0.0672&0.4313&0.5843&0.6667&0.8760\\
RNN+&0.0736&0.4604&0.6136&\textbf{0.6930}&0.8785\\
RNN&0.0733&0.4478&0.6103&0.6921&0.8767\\
SimpleRollUp&0.0662&\textbf{0.4924}&\textbf{0.6312}&0.6907&0.8795\\
RollUpRare&0.0759&0.4657&0.6146&0.6908&0.8778\\
\bottomrule
\end{tabular}
\caption{\textit{Accuracy@30} of sequential diagnoses prediction on Sutter data}
\label{tab:sdp_sutter_30}
\end{subtable}

\caption{Accuracy at various $k$'s (a to d) for sequential diagnoses prediction on Sutter data. The columns represent the labels grouped by the percentile of their frequencies in the training data in non-decreasing order.}
\label{tab:sutter_dpm}
\end{table*}
\begin{table*}
\centering
\small
%\vspace*{-2mm}
\begin{subtable}{1.\textwidth}
\centering
\begin{tabular}{l|c|c|c|c|c}
Model & 0-20 & 20-40 & 40-60 & 60-80 & 80-100\\ 
\toprule
GRAM+&\textbf{0.0086}&\textbf{0.1089}&\textbf{0.1665}&0.1029&0.2597\\
GRAM&0.0000&0.0468&0.1093&0.0918&\textbf{0.2665}\\
RandomDAG&0.0000&0.0327&0.0778&0.0612&0.1634\\
RNN+&0.0000&0.0435&0.1266&0.0973&0.2594\\
RNN&0.0000&0.0376&0.1105&0.0923&0.2601\\
SimpleRollUp&0.0000&0.0671&0.1501&\textbf{0.1191}&0.2635\\
RollUpRare&0.0000&0.0423&0.1085&0.0874&0.2604\\
\bottomrule
\end{tabular}
\caption{\textit{Accuracy@5} of sequential diagnoses prediction on MIMIC-III}
\label{tab:sdp_mimic_5}
\end{subtable}

\begin{subtable}{1.\textwidth}
\centering
\begin{tabular}{l|c|c|c|c|c}
Model & 0-20 & 20-40 & 40-60 & 60-80 & 80-100\\ 
\toprule
GRAM+&\textbf{0.0380}&\textbf{0.1310}&\textbf{0.2095}&0.1627&0.4175\\
GRAM&0.0045&0.0682&0.1494&0.1487&0.4235\\
RandomDAG&0.0023&0.0470&0.1025&0.0938&0.2692\\
RNN+&0.0227&0.0587&0.1591&0.1616&0.4193\\
RNN&0.0023&0.0518&0.1389&0.1521&0.4142\\
SimpleRollUp&0.0249&0.1038&0.1997&\textbf{0.1769}&\textbf{0.4260}\\
RollUpRare&0.0227&0.0530&0.1412&0.1519&0.4180\\
\bottomrule
\end{tabular}
\caption{\textit{Accuracy@10} of sequential diagnoses prediction on MIMIC-III}
\label{tab:sdp_mimic_10}
\end{subtable}

\begin{subtable}{1.\textwidth}
\centering
\begin{tabular}{l|c|c|c|c|c}
Model & 0-20 & 20-40 & 40-60 & 60-80 & 80-100\\ 
\toprule
GRAM+&\textbf{0.0672}&\textbf{0.1787}&\textbf{0.2644}&0.2490&0.6267\\
GRAM&0.0556&0.1016&0.1935&0.2296&0.6363\\
RandomDAG&0.0329&0.0708&0.1346&0.1512&0.4494\\
RNN+&0.0454&0.0843&0.2080&0.2494&0.6239\\
RNN&0.0454&0.0731&0.1804&0.2371&0.6243\\
SimpleRollUp&0.0578&0.1328&0.2455&\textbf{0.2667}&\textbf{0.6387}\\
RollUpRare&0.0454&0.0653&0.1843&0.2364&0.6277\\
\bottomrule
\end{tabular}
\caption{\textit{Accuracy@20} of sequential diagnoses prediction on MIMIC-III}
\label{tab:sdp_mimic_20}
\end{subtable}

\begin{subtable}{1.\textwidth}
\centering
\begin{tabular}{l|c|c|c|c|c}
Model & 0-20 & 20-40 & 40-60 & 60-80 & 80-100\\ 
\toprule
GRAM+&\textbf{0.0744}&\textbf{0.2065}&\textbf{0.3180}&0.3363&0.7726\\
GRAM&0.0578&0.1157&0.2257&0.3074&\textbf{0.7802}\\
RandomDAG&0.0351&0.0932&0.1635&0.2200&0.5977\\
RNN+&0.0578&0.1103&0.2571&0.3409&0.7656\\
RNN&0.0578&0.0775&0.2237&0.3160&0.7643\\
SimpleRollUp&0.0578&0.1556&0.2865&\textbf{0.3488}&0.7800\\
RollUpRare&0.0556&0.0910&0.2235&0.3255&0.7661\\
\bottomrule
\end{tabular}
\caption{\textit{Accuracy@30} of sequential diagnoses prediction on MIMIC-III}
\label{tab:sdp_mimic_30}
\end{subtable}

\caption{Accuracy at various $k$'s (a to d) for sequential diagnoses prediction on MIMIC-III. The columns represent the labels grouped by the percentile of their frequencies in the training data in non-decreasing order.}
\label{tab:mimic_dpm}
\end{table*}

We show $Accuracy@k$ using $k=5,10,20,30$ for sequential diagnoses prediction on Sutter data (Tables \ref{tab:sdp_sutter_5}, \ref{tab:sdp_sutter_10}, \ref{tab:sdp_sutter_20} and \ref{tab:sdp_sutter_30}) and MIMIC-III (Tables \ref{tab:sdp_mimic_5}, \ref{tab:sdp_mimic_10}, \ref{tab:sdp_mimic_20} and \ref{tab:sdp_mimic_30}). We can see from the tables that \texttt{GRAM}+ consistently outperforms other models under 40th percentile range, except when $k=20,30$ for sequential diagnoses prediction on Sutter data where SimpleRollUp shows similar performance. We can also see that \texttt{GRAM}+ performs significantly better than other models for all $k=5,10,20,30$ when predicting infrequently observed diseases on MIMIC-III. As discussed in Section \ref{ssec:exp_prediction}, this seems to come from the short visit sequences of MIMIC patients.

\section{t-SNE 2-D Plots of Various Models}
\label{appendix:tsne}
\begin{figure*}
\centering
\begin{subfigure}{.5\textwidth}
  \centering\captionsetup{width=.9\linewidth}%
  \includegraphics[width=.9\linewidth]{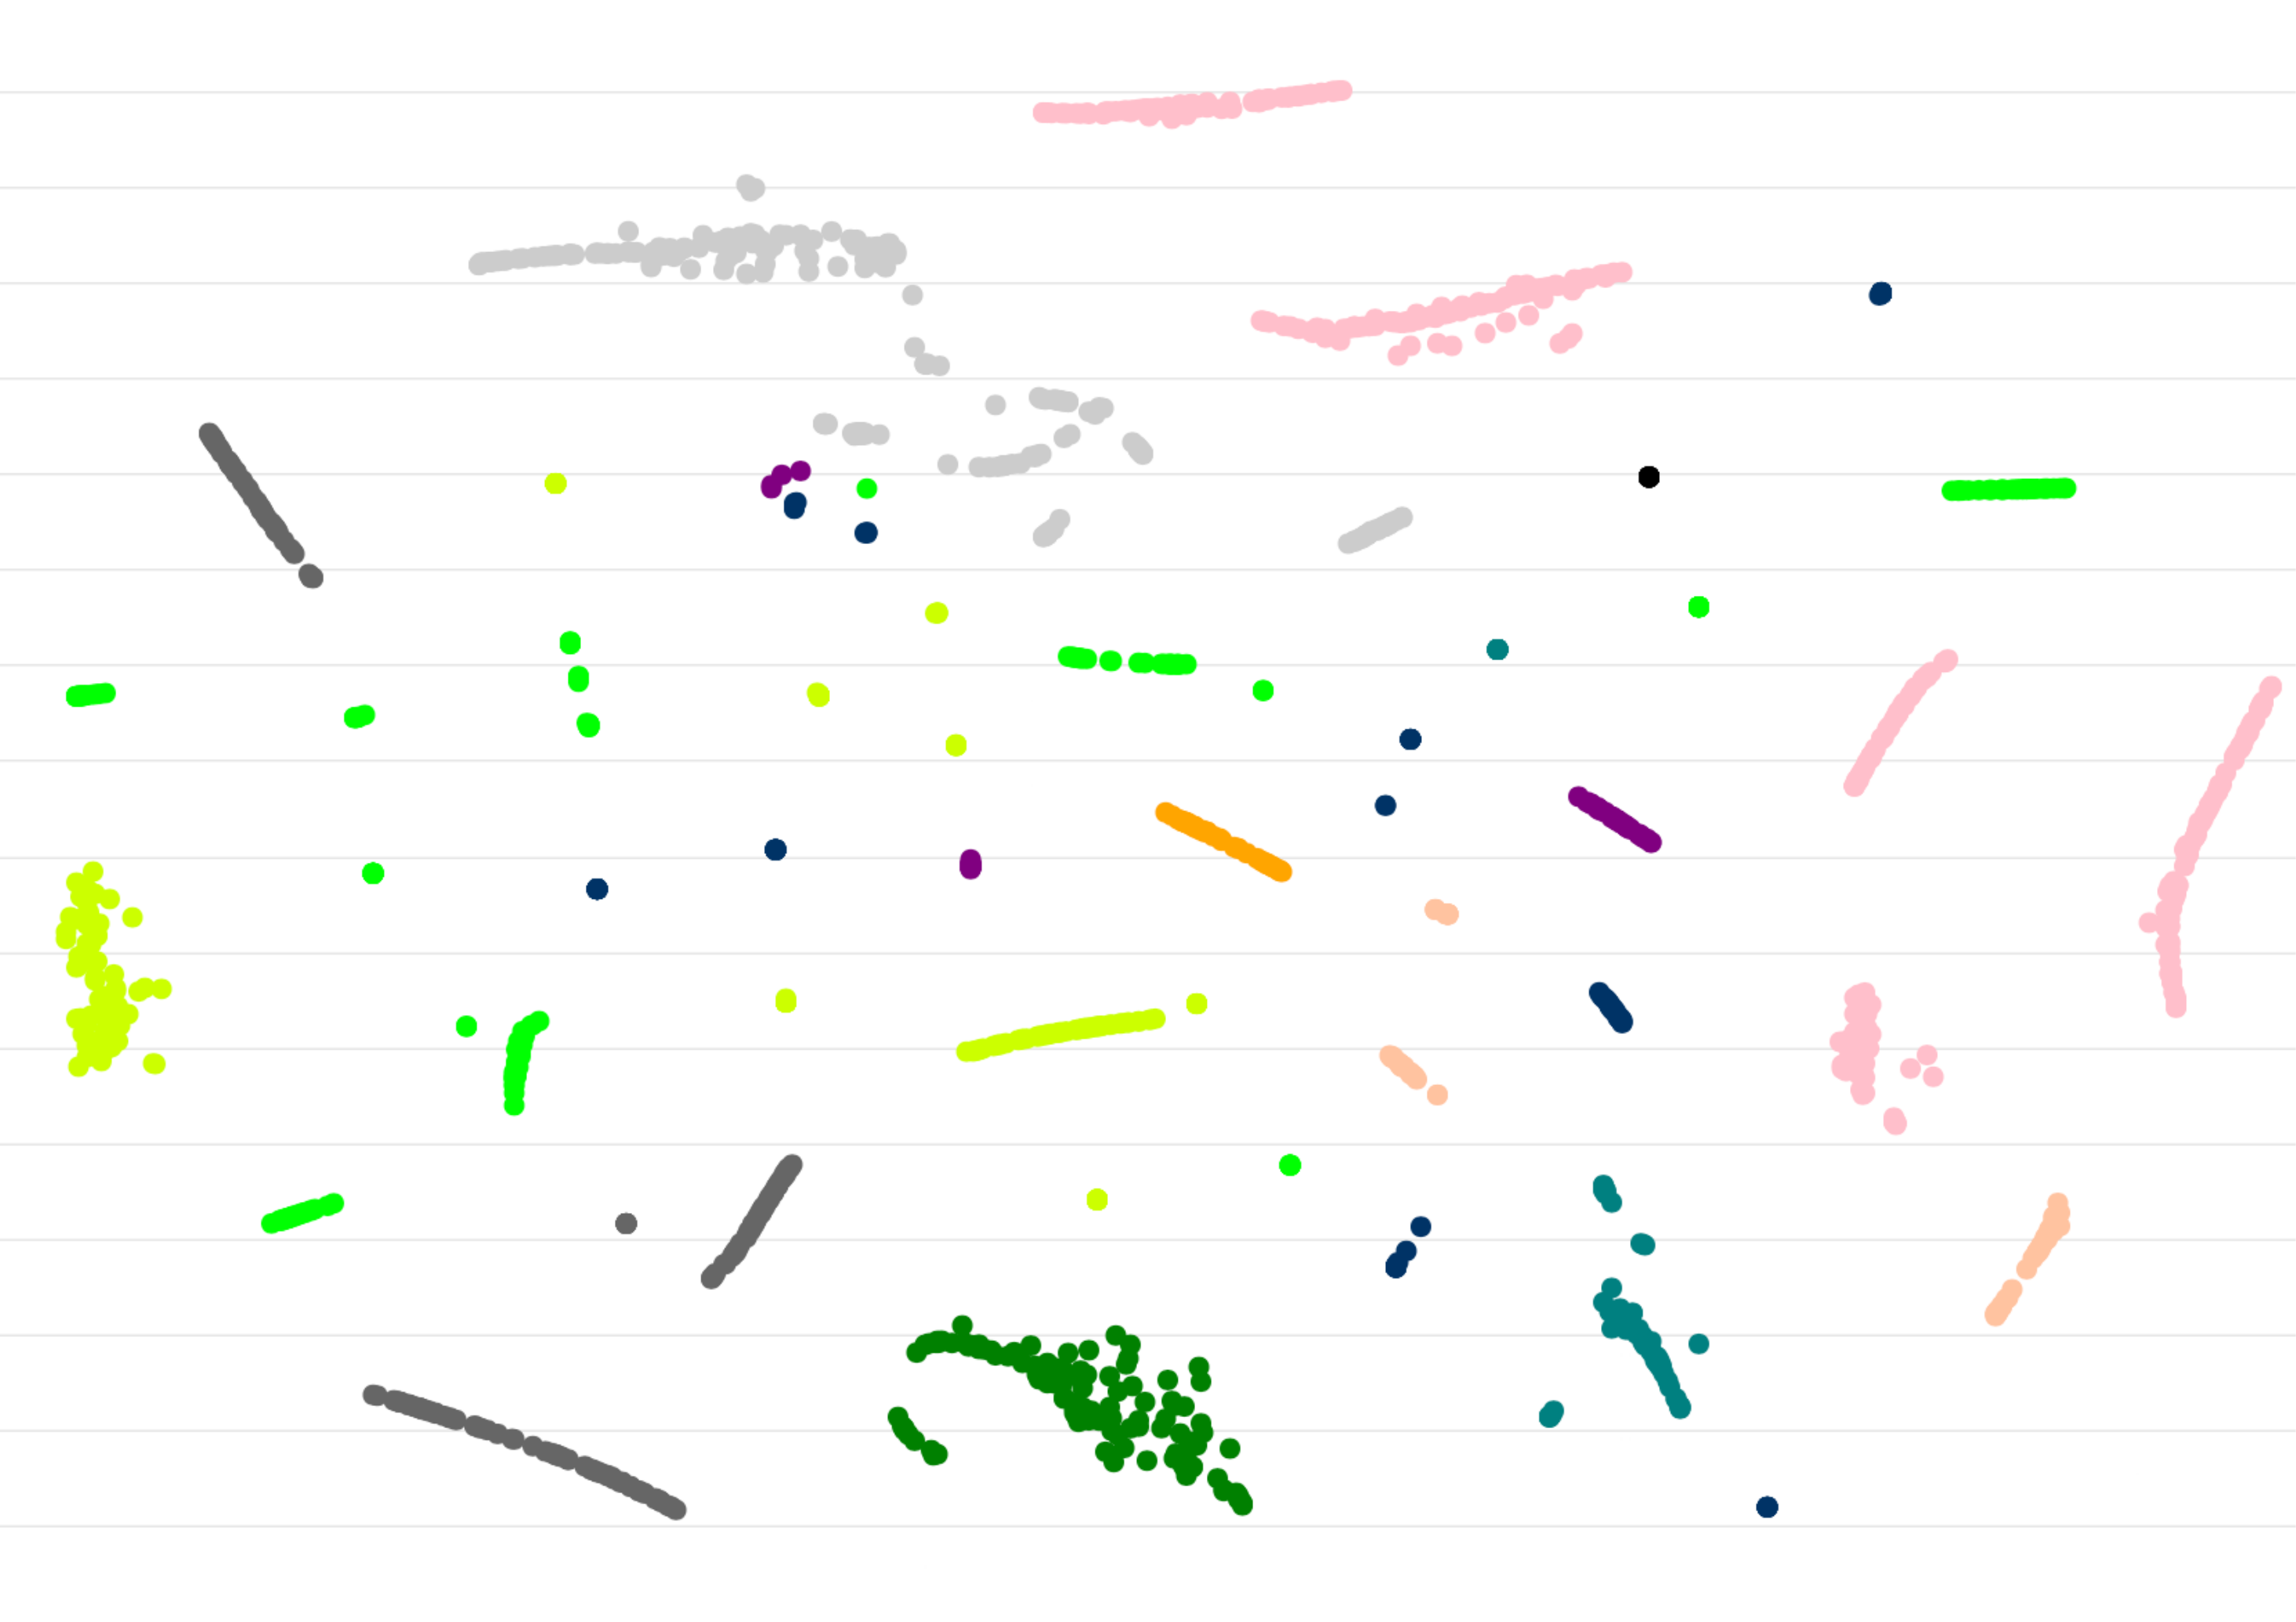}
  \caption{Scatterplot of the final representations $\gb_i$'s of \mname}
  \label{fig:tsne_alg}
\end{subfigure}%
\begin{subfigure}{.5\textwidth}
  \centering\captionsetup{width=.9\linewidth}%
  \includegraphics[width=.9\linewidth]{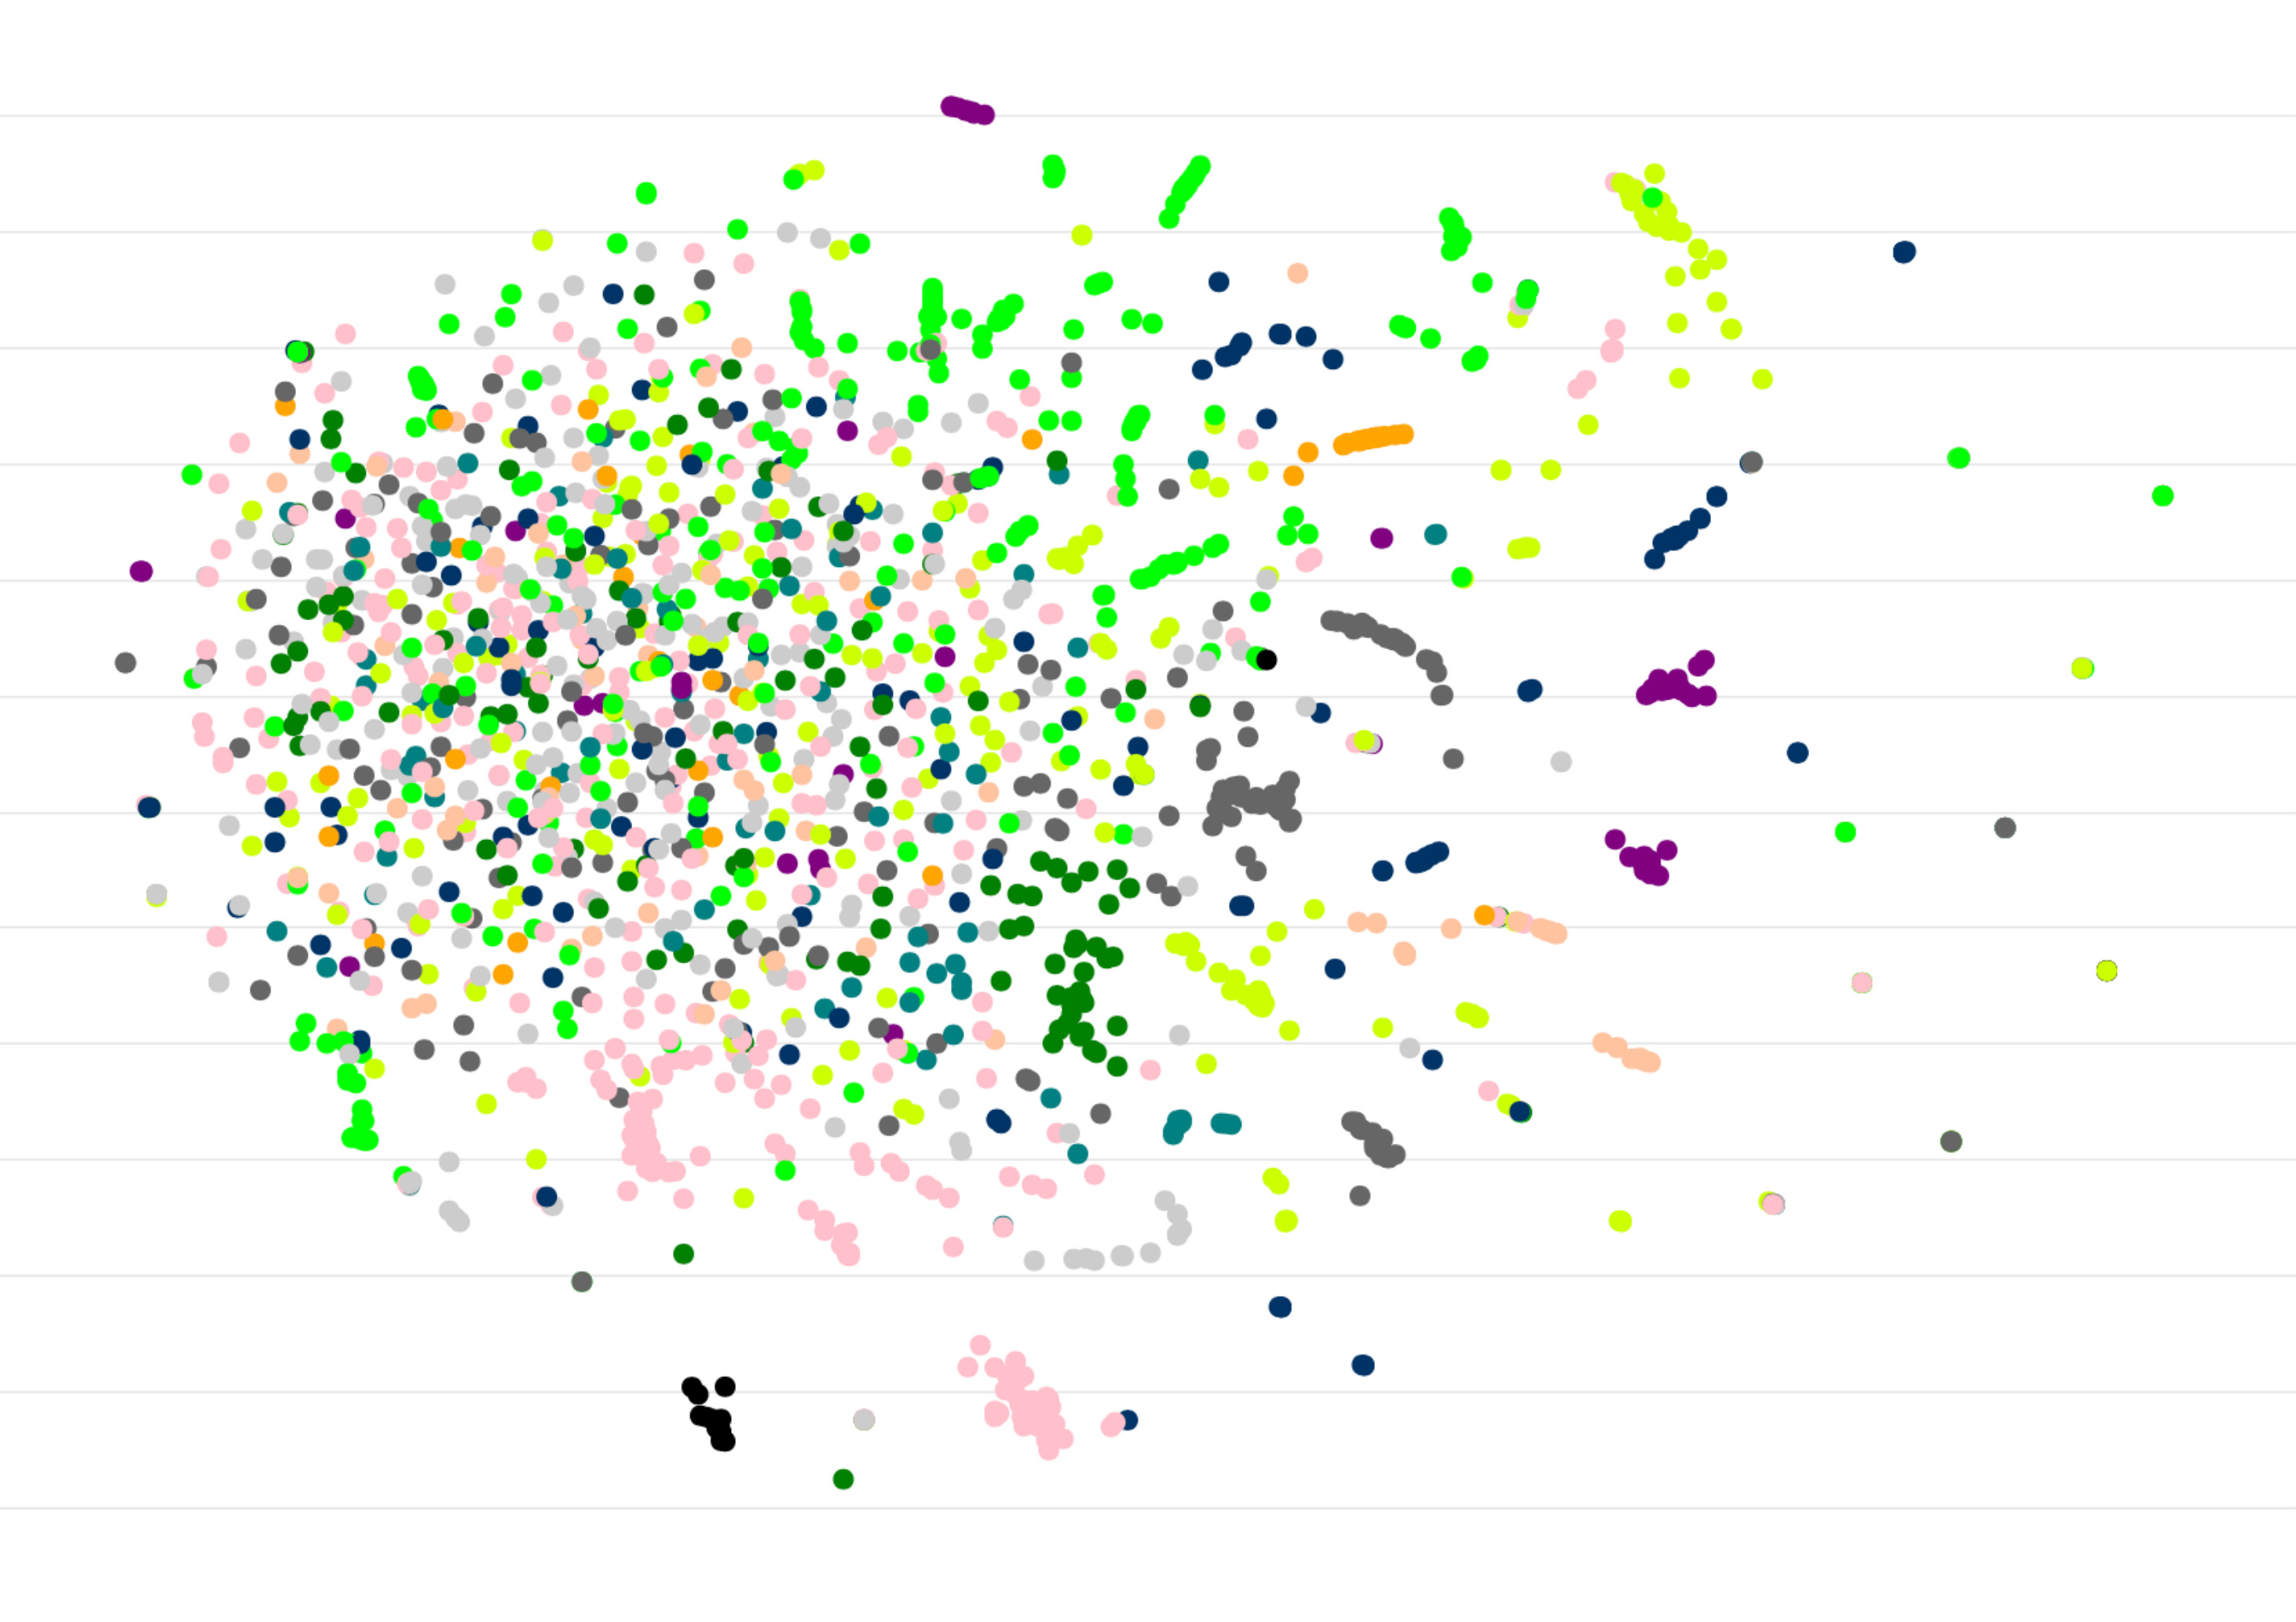}
  \caption{Scatterplot of the final representations $\gb_i$'s of RandomDAG}
  \label{fig:tsne_alg_fake}
\end{subfigure}

\begin{subfigure}{.5\textwidth}
  \centering\captionsetup{width=.9\linewidth}%
  \includegraphics[width=.9\linewidth]{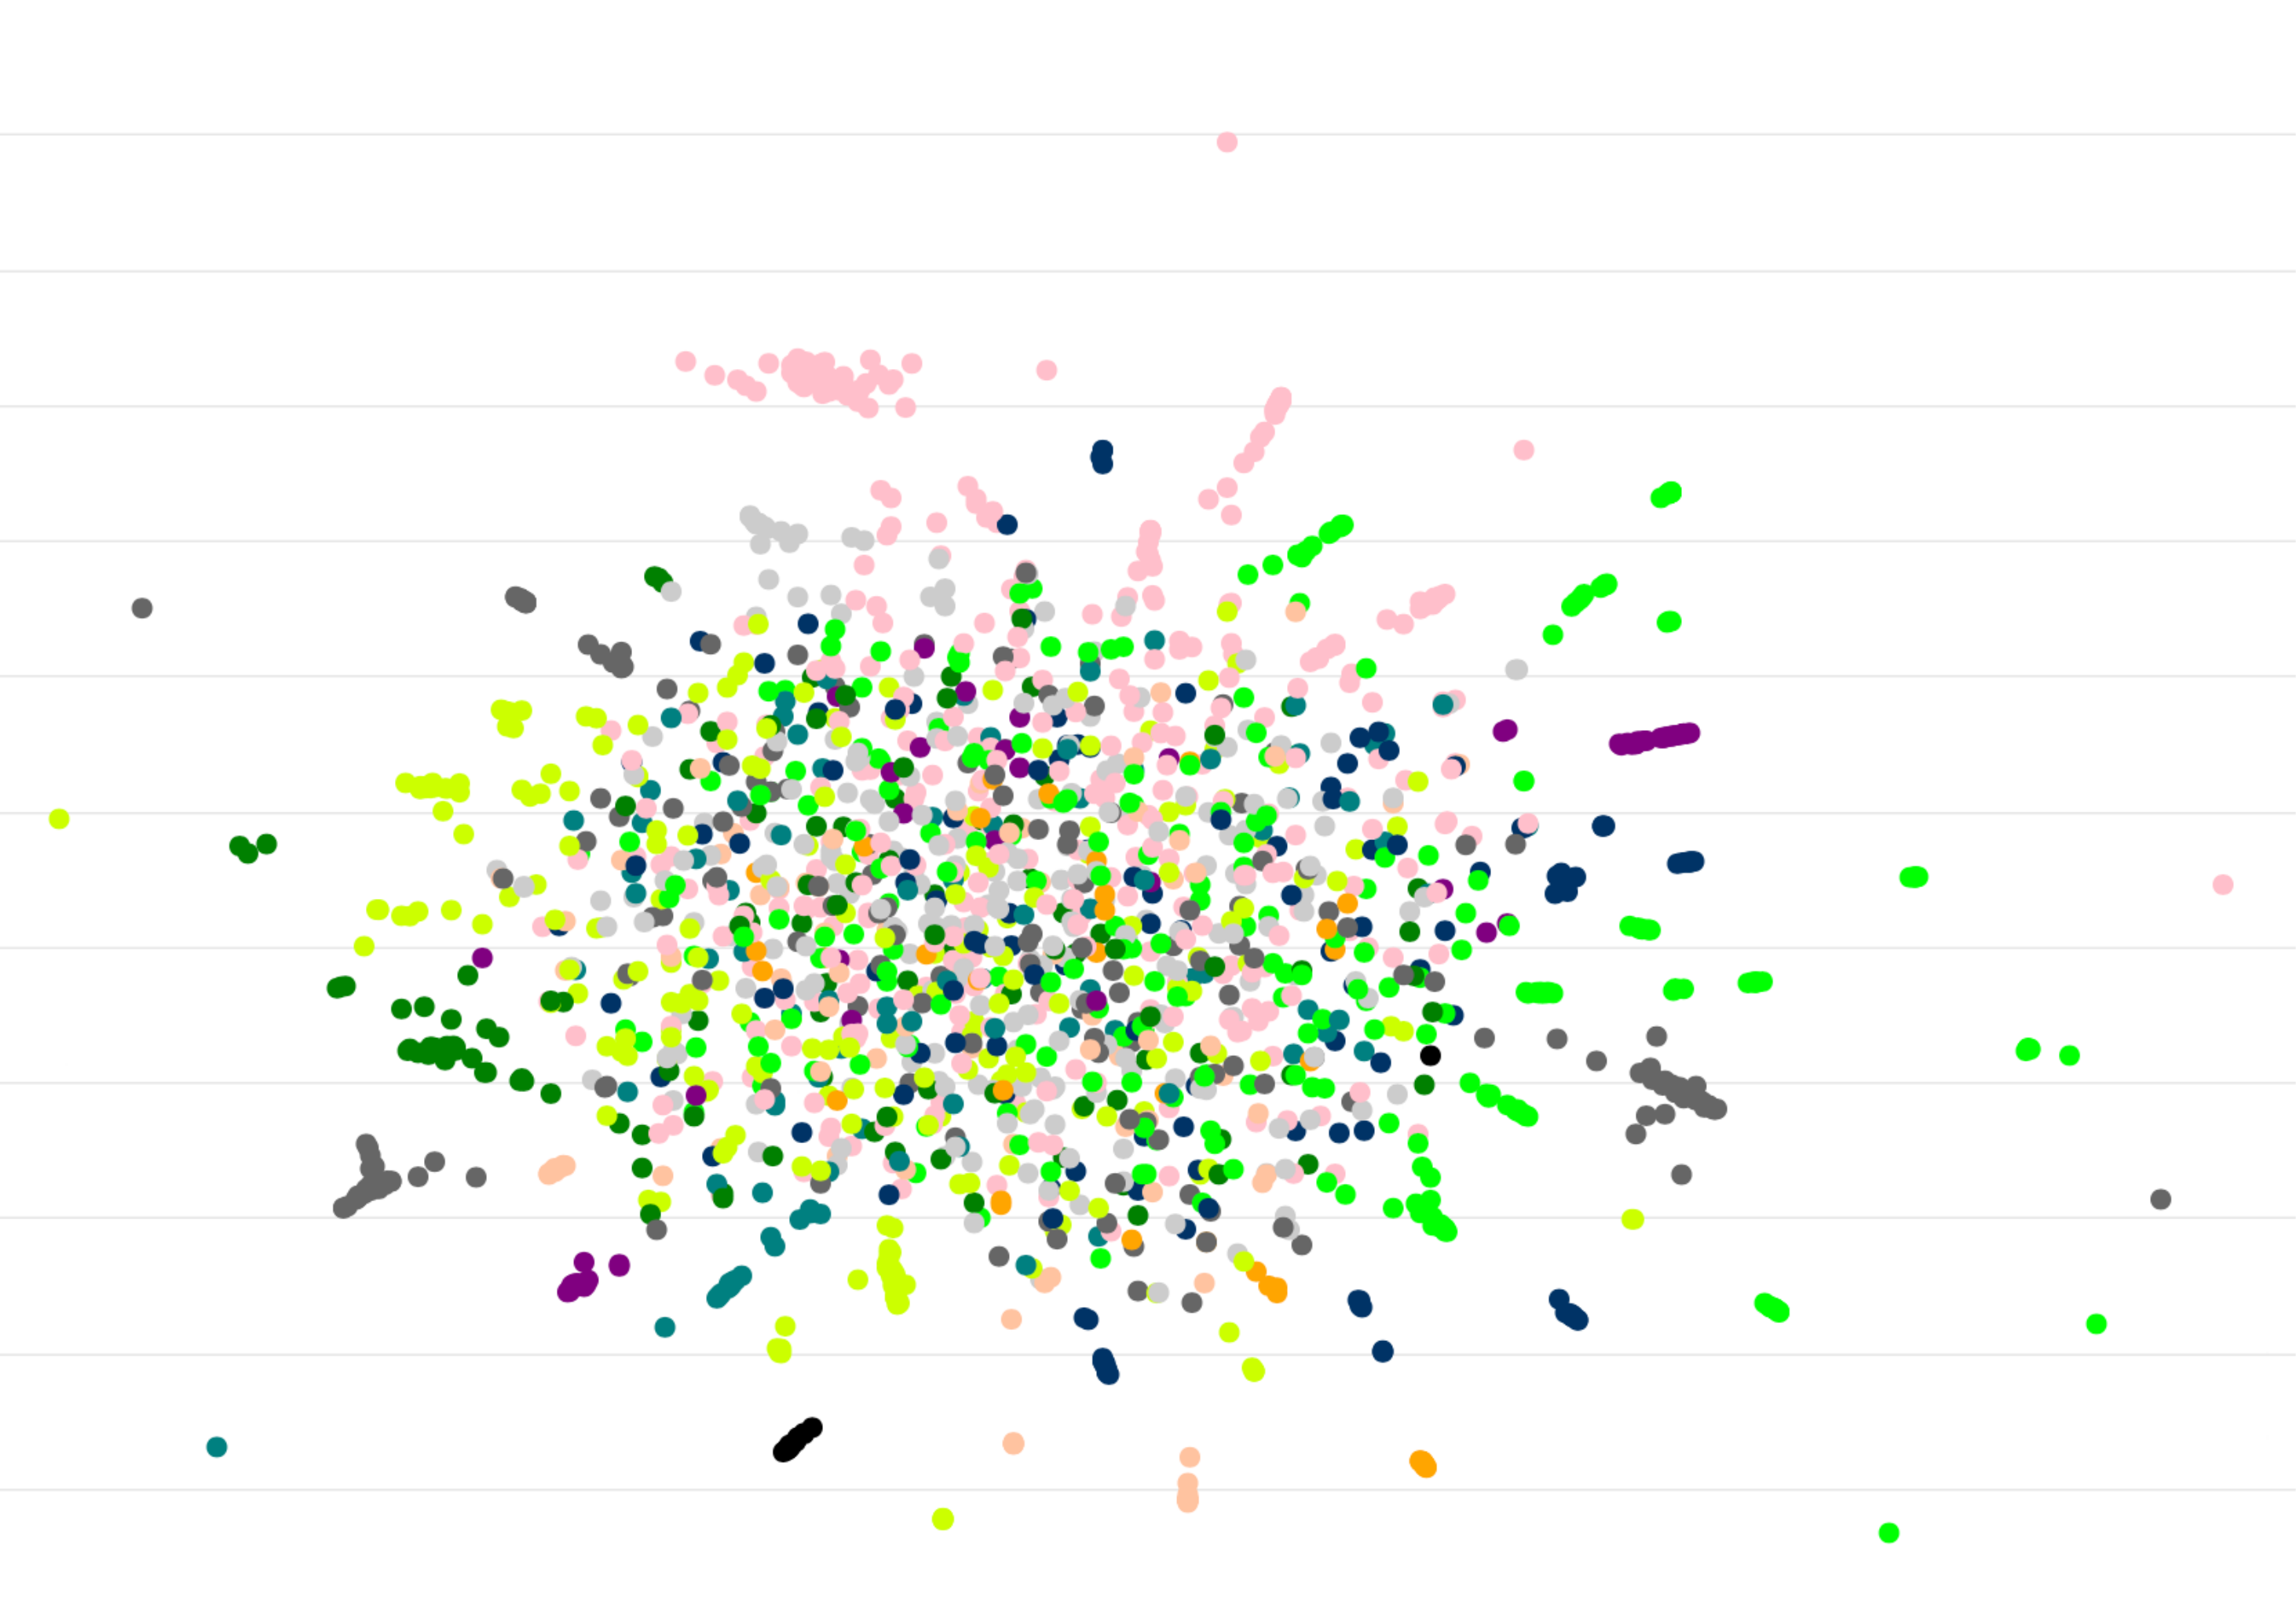}
  \caption{Scatterplot of the trained embedding matrix $\Wb_{emb}$ of RNN}
  \label{fig:tsne_rnn}
\end{subfigure}%
\begin{subfigure}{.5\textwidth}
  \centering\captionsetup{width=.9\linewidth}%
  \includegraphics[width=.9\linewidth]{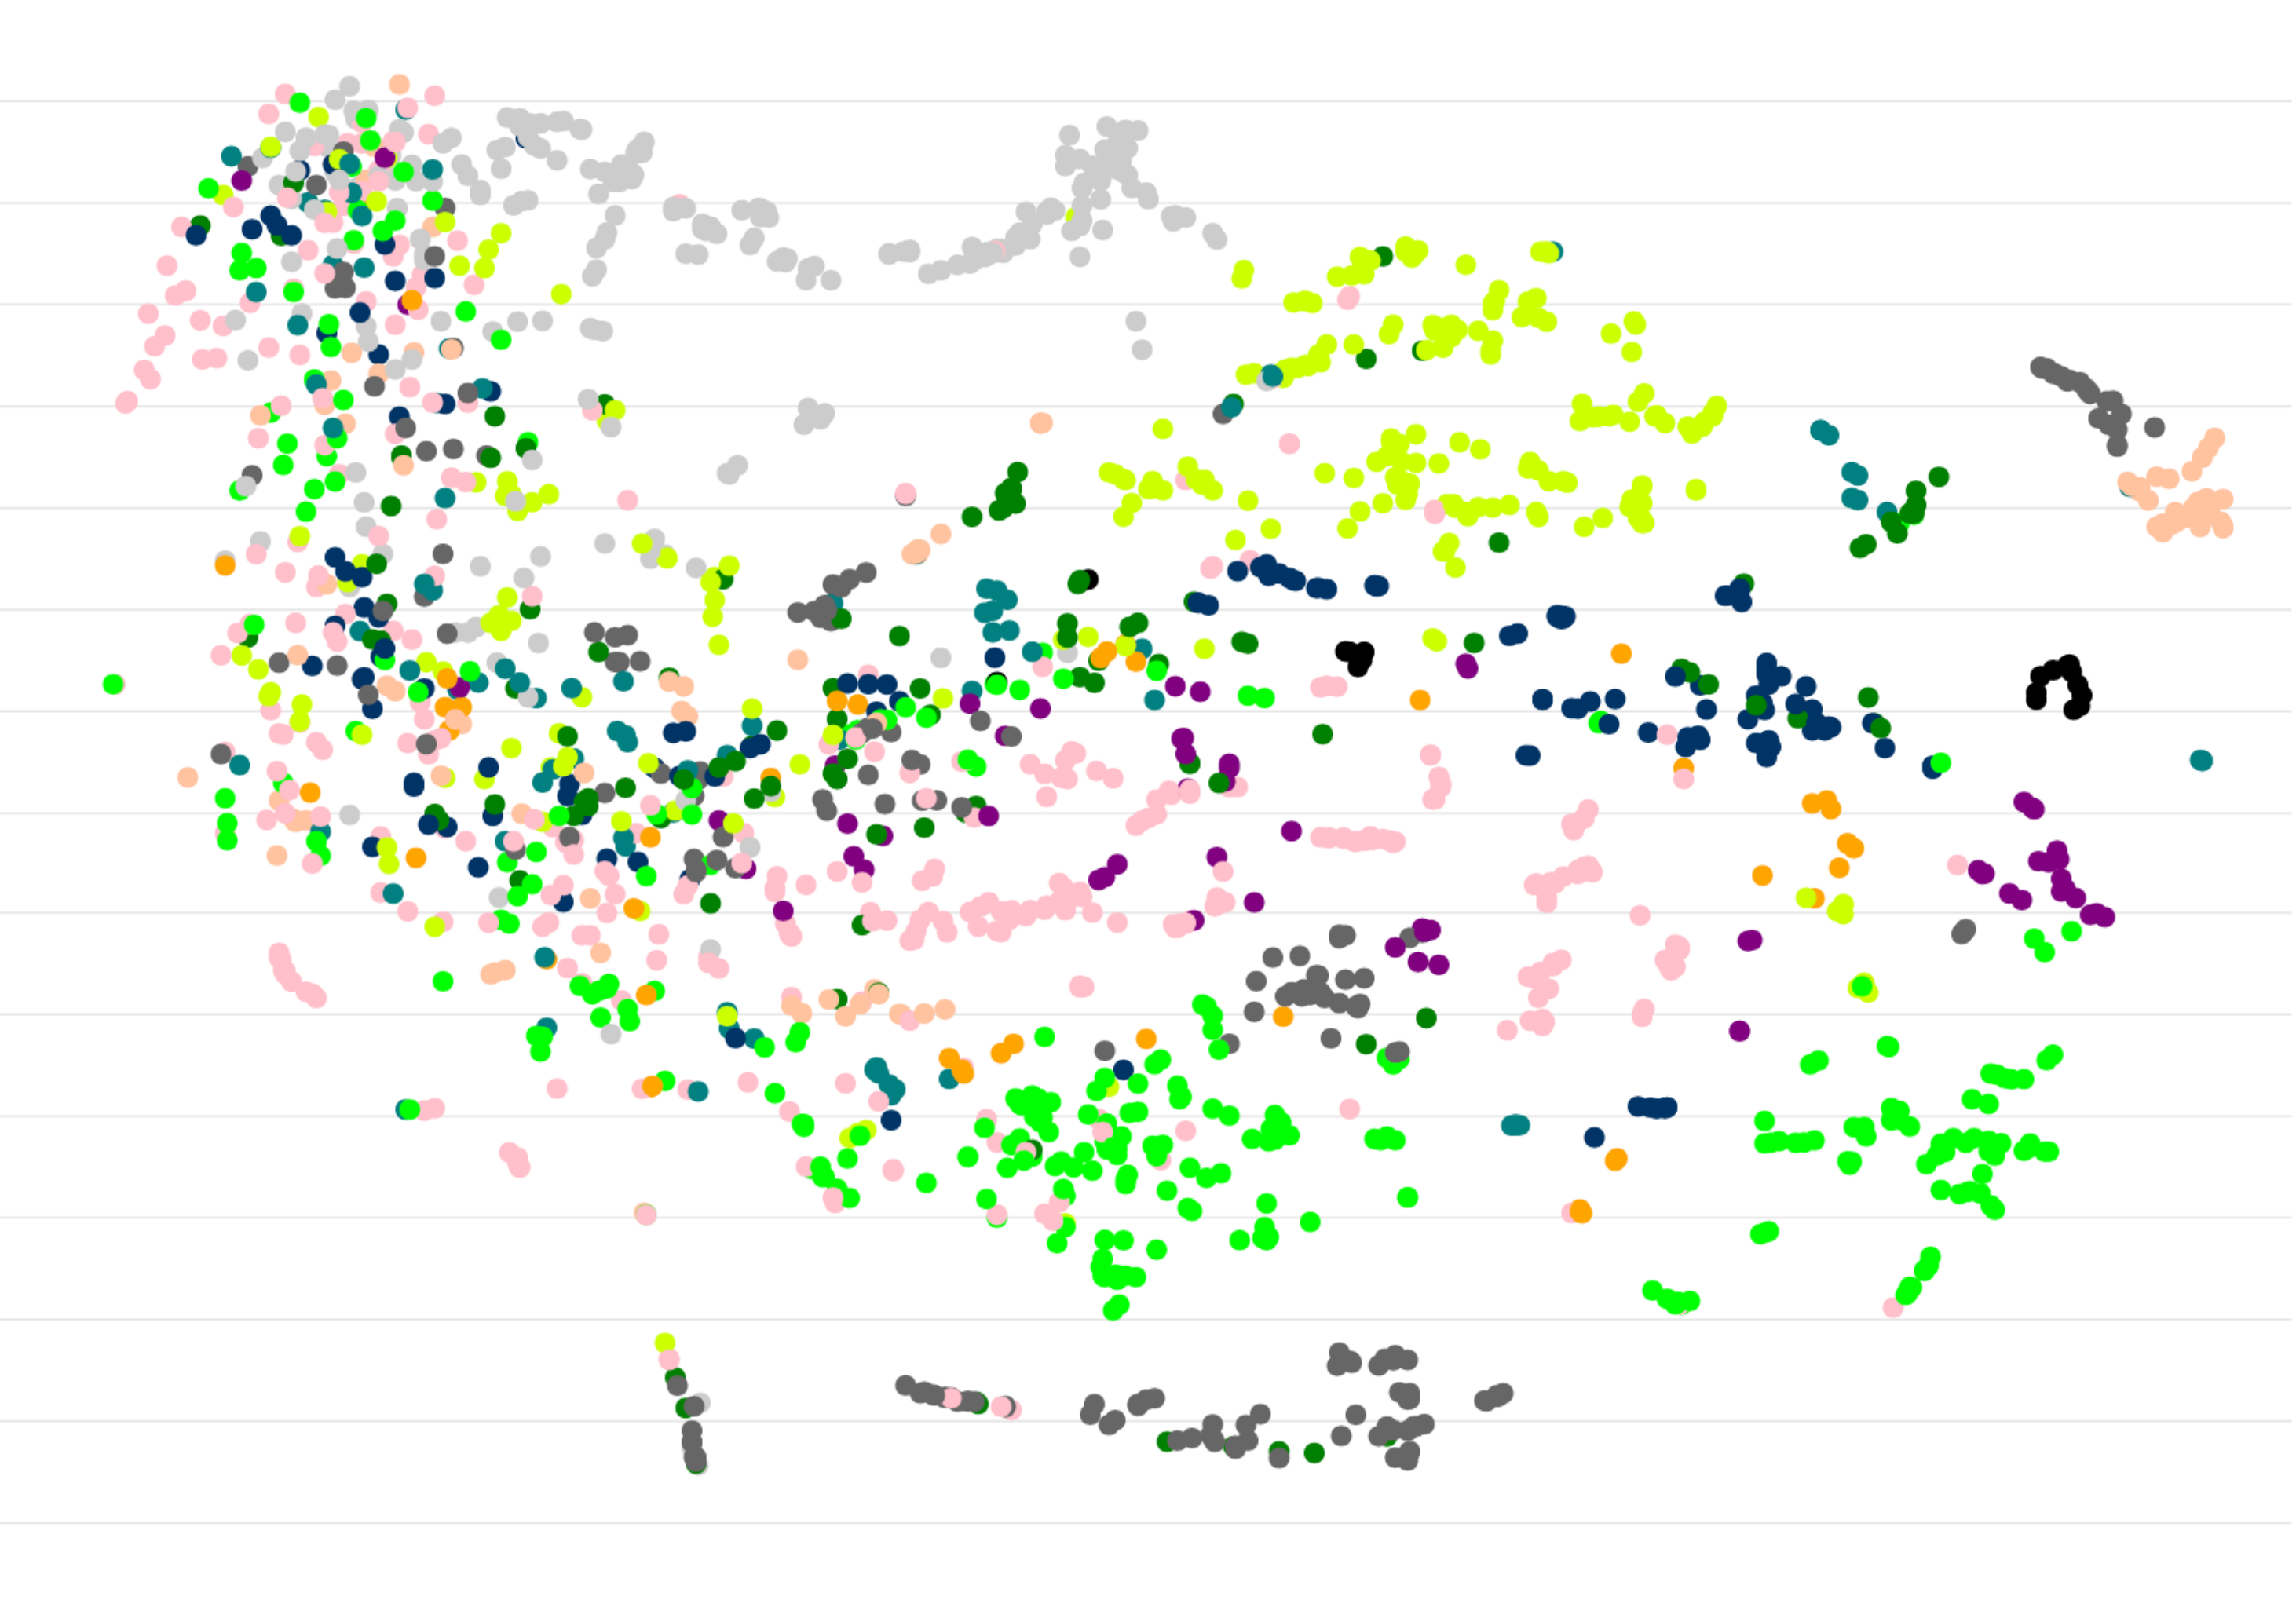}
  \caption{Scatterplot of the basic embeddings $\eb_i$'s trained by Skip-gram}
  \label{fig:tsne_skipgram}
\end{subfigure}
\caption{Scatterplot of medical concepts trained by various models. We used t-SNE to reduce the dimension to 2-D.}
\label{fig:tsne}
\end{figure*}

For further comparison, we display t-SNE scatterplots of \mname (Figure \ref{fig:tsne_alg}) RandomDAG (Figure \ref{fig:tsne_alg_fake}, RNN (Figure \ref{fig:tsne_rnn}), and Skip-gram (Figure \ref{fig:tsne_skipgram}). \mname, RandomDAG and RNN were trained for sequential diagnoses prediction on Sutter data, and Skip-gram \citep{mikolov2013distributed} was trained on Sutter data as it is an unsupervised method. For Skip-gram, we used each visit $V_t$ as the context window. As we do not distinguish between the target concept and the neighbor concepts, we calculated the Skip-gram objective function using all possible pairs of codes within a single visit. 

We can see from Figure \ref{fig:tsne_alg} that the quality of the final representations $\gb_i$ of \mname is quite similar to \texttt{GRAM}+ (Figure \ref{fig:tsne_alg_glove}). Compared to other baselines, \mname demonstrates significantly more structured representations that align well with the given knowledge DAG. It is interesting that Skip-gram shows the most structured representation among all baselines. We used GloVe to initialize the basic embeddings $\eb_i$ in this work because it uses global co-occurrence information and its training time is dependent only on the total number of unique concepts $|\mathcal{C}|$. Skip-gram's training time, on the other hand, depends on both the number of patients and the number of visits each patient made, which makes the algorithm generally slower than GloVe. However, considering both Figures \ref{fig:tsne_glove} and \ref{fig:tsne_skipgram}, initializing $\eb_i$'s with Skip-gram vectors might give us additional performance boost.

% \section{Statistical Results of Attention Behavior Analysis}
% \label{appendix:attention}
%\input{old_exp_attention.tex}
